# Supplementary material for: FedDRL: Deep Reinforcement Learning-based Adaptive Aggregation for Non-IID Data in Federated Learning
Source: arXiv:2208.02442 source file (2022-08-04)
Supplement: Supplementary file 1 [file 08_appendix.tex]

%% Appendix
\newpage
\appendix
\section{APPENDIX}\label{appendix}
\subsection{Extra Result}
\begin{figure*}
     \centering
     \small
     \subfigure[Fashion-MNIST, Cluster-E partitioning, 10 clients.]{
        \label{fig:fmnist_level10_f}
        \includegraphics[width=1\linewidth]{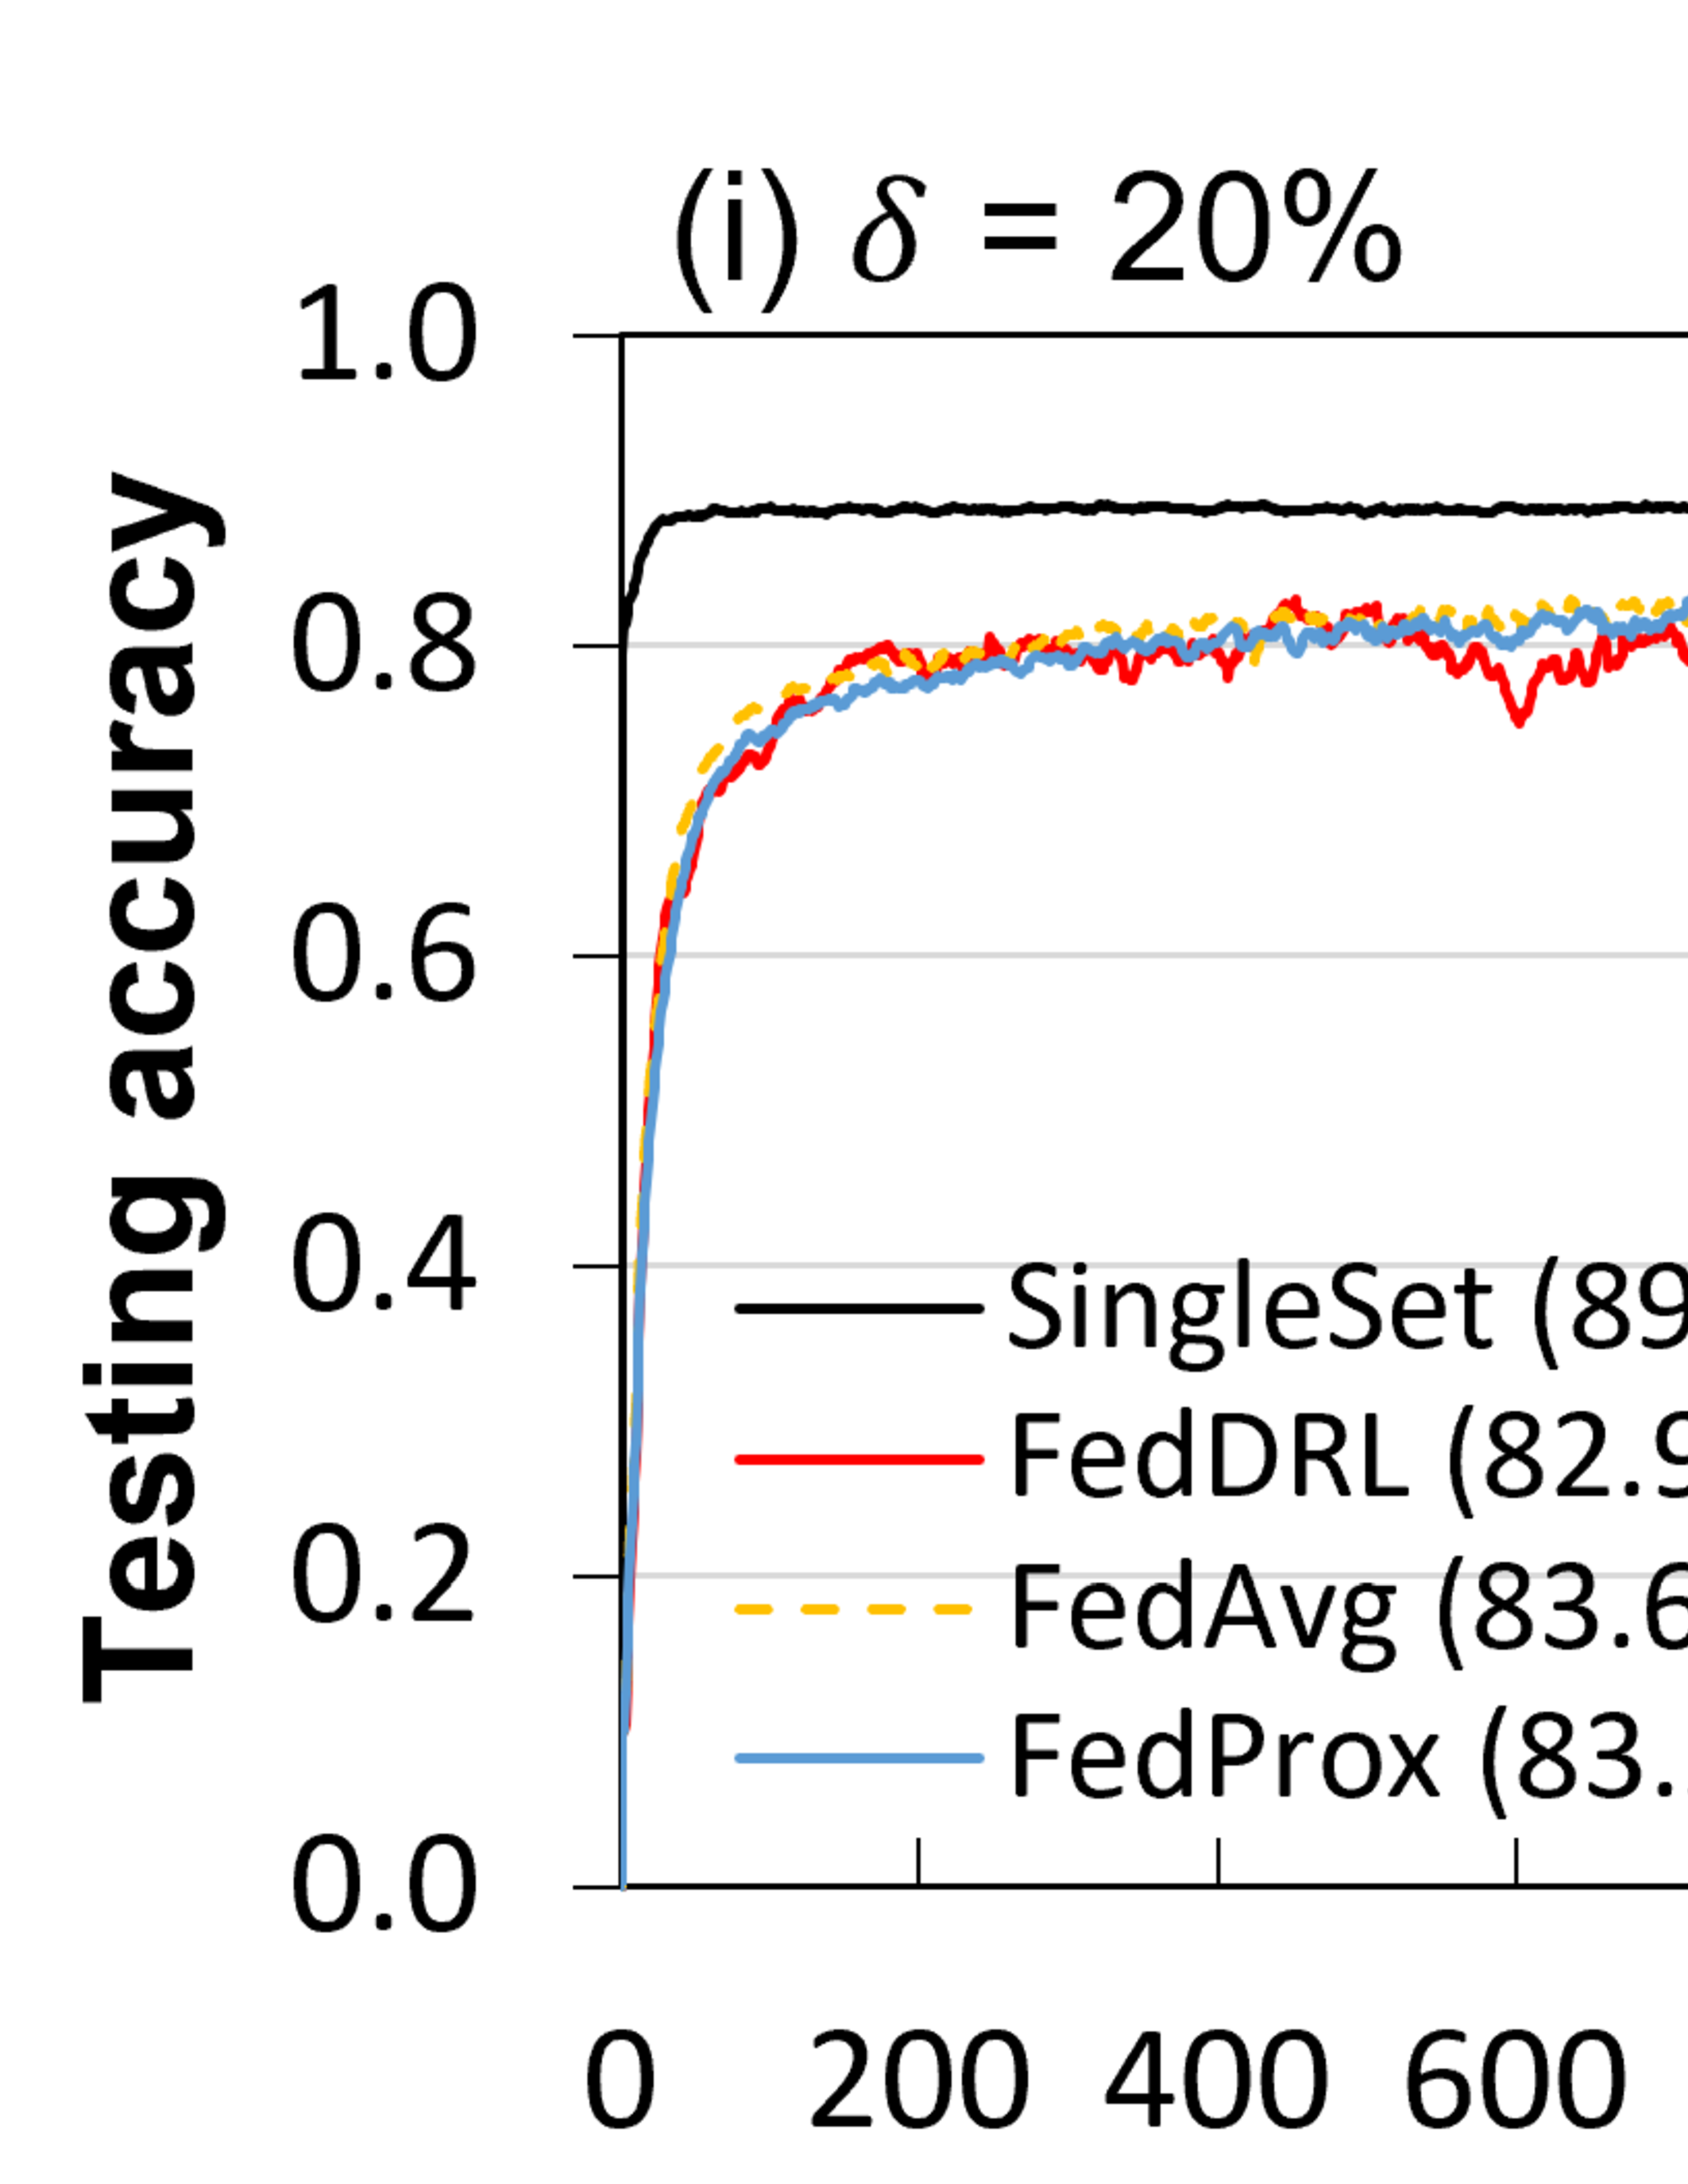}
     }
      \subfigure[Fashion-MNIST, Cluster-NE partitioning, 10 clients.]{
        \label{fig:fmnist_level10_q}
        \includegraphics[width=1\linewidth]{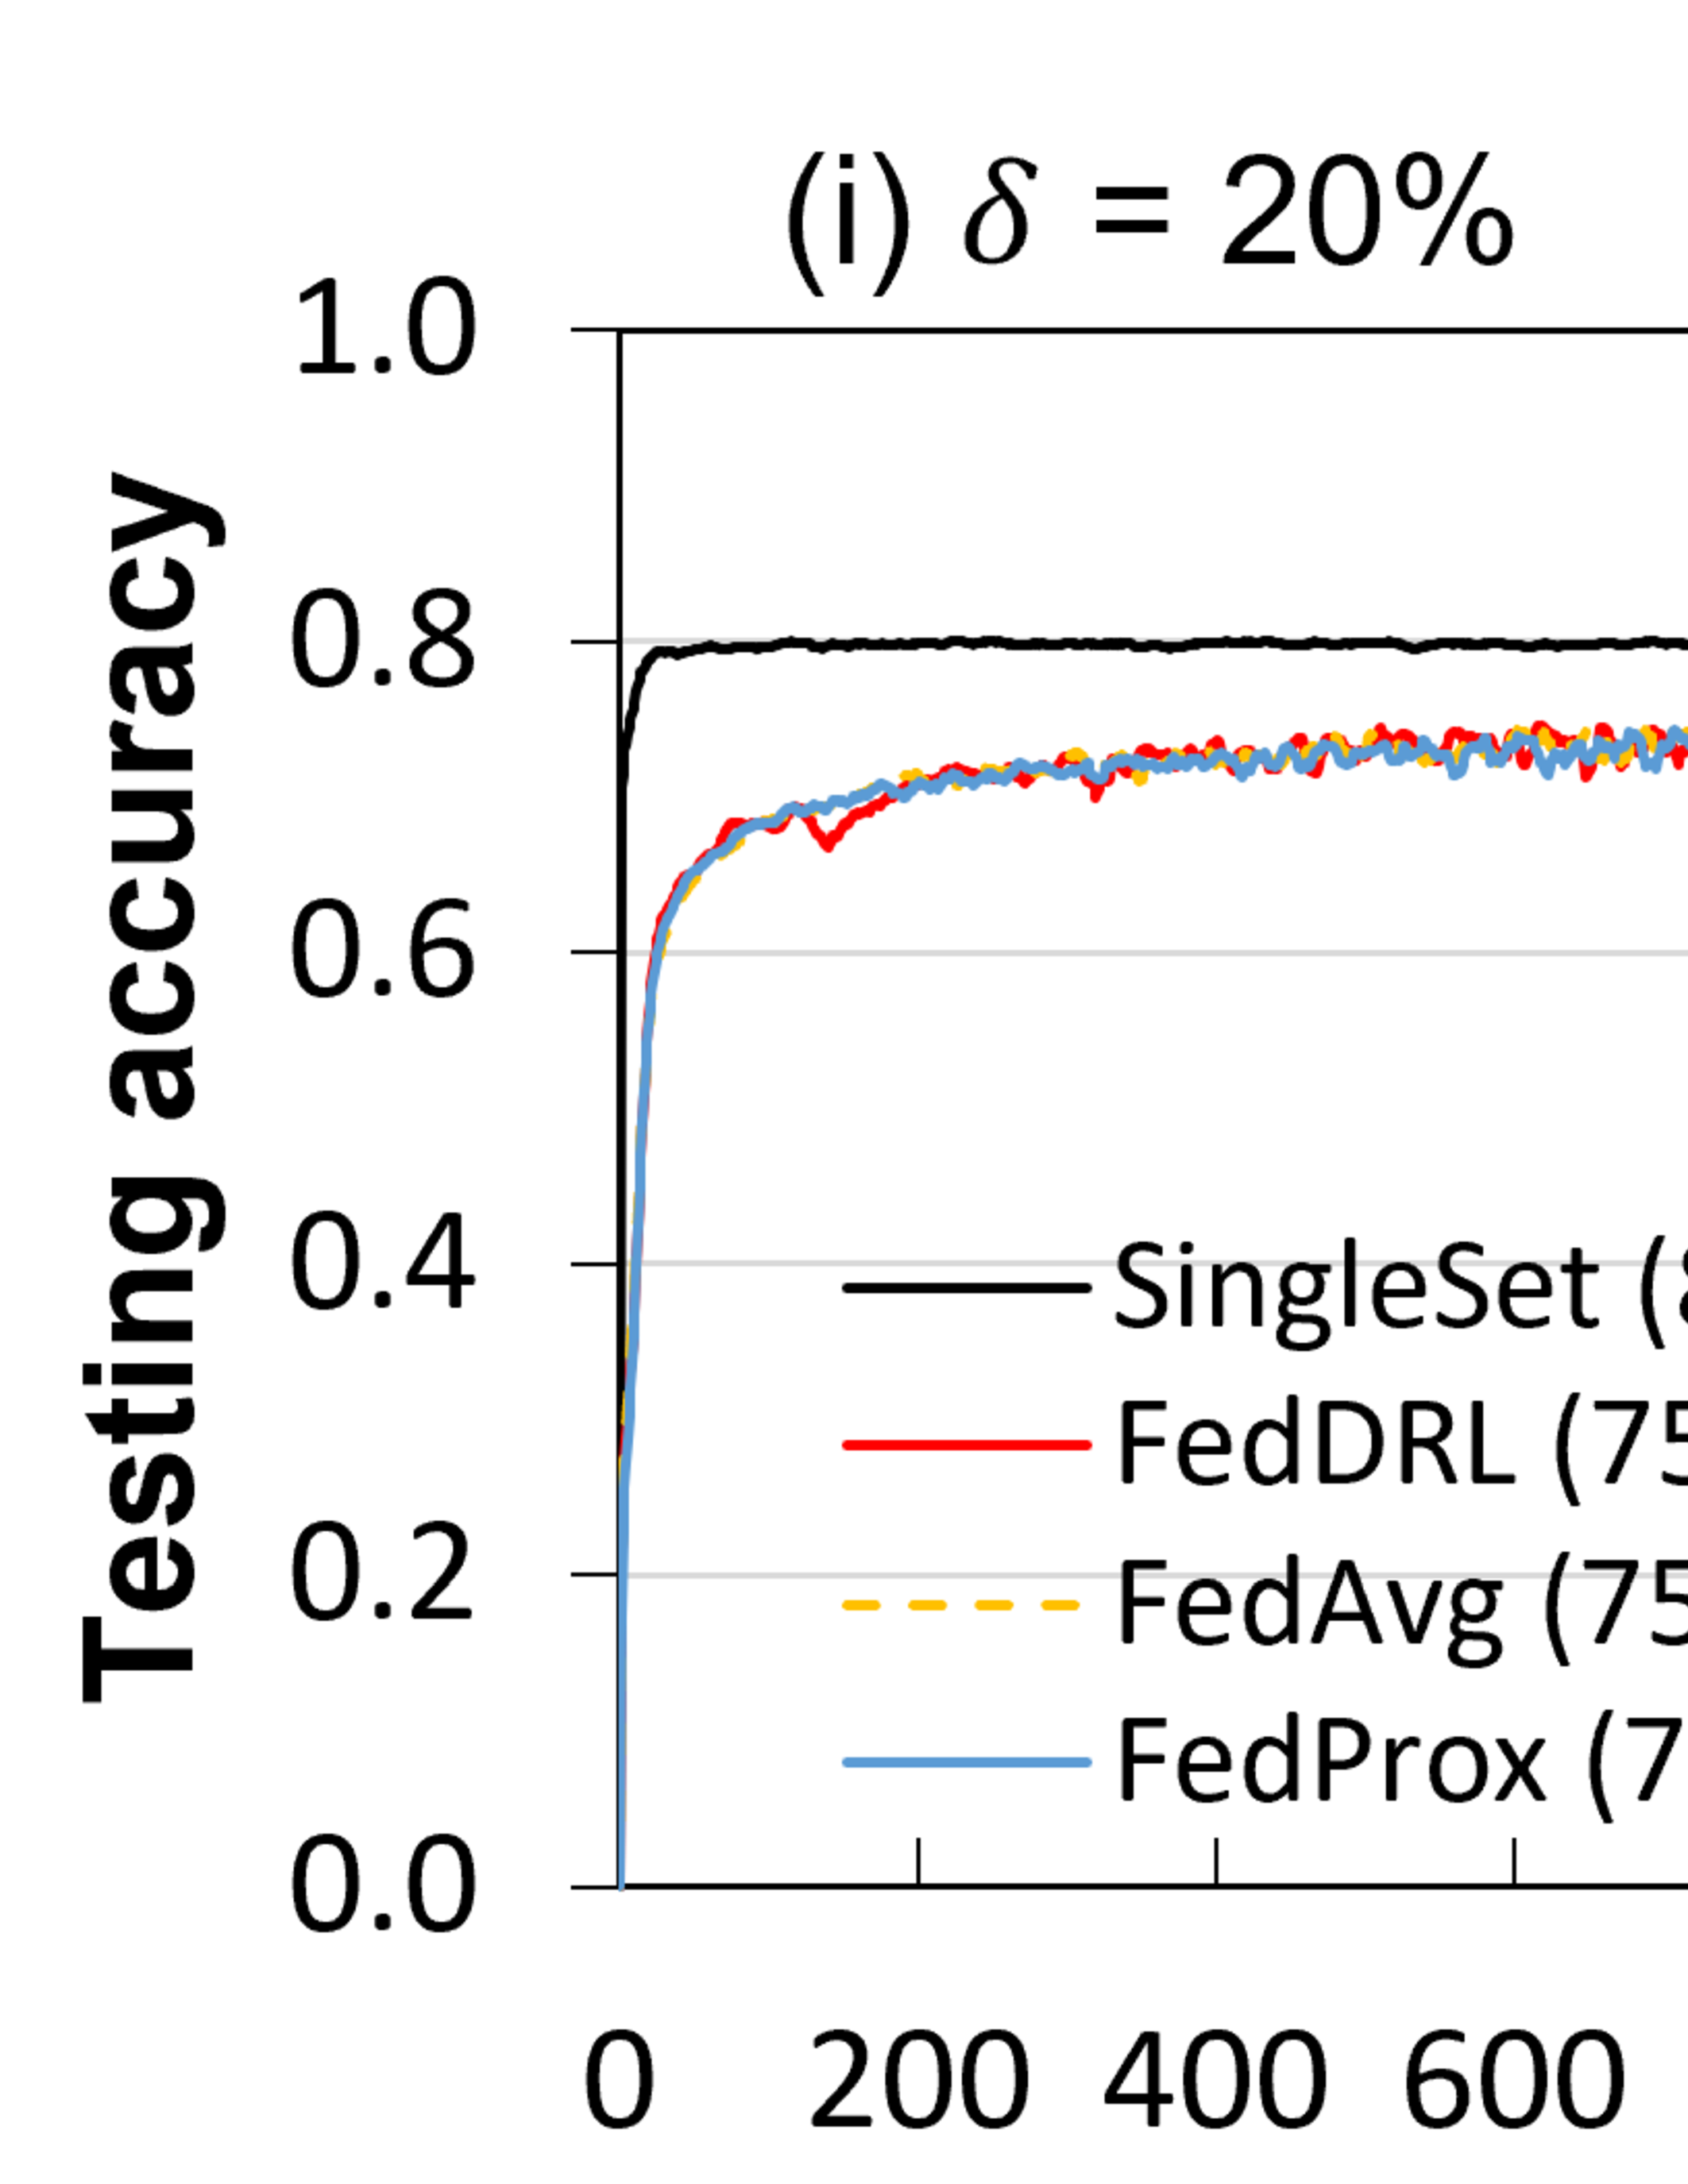}
     }
     \caption{Testing accuracy \textit{vs.} the non-IID level $\delta$ in the case of Fashion-MNIST, 10 clients. The X-axis is communication round. The results are average-smoothed for every $10$ communication round. The values in the legends show the best testing accuracy that each FL methods reach during training.}
     \label{fig:fmnist_level10}
 \end{figure*}
 \begin{figure*}
     \centering
     \small
     \subfigure[Fashion-MNIST, Cluster-E partitioning, 100 clients.]{
        \label{fig:fmnist_level100_f}
        \includegraphics[width=1\linewidth]{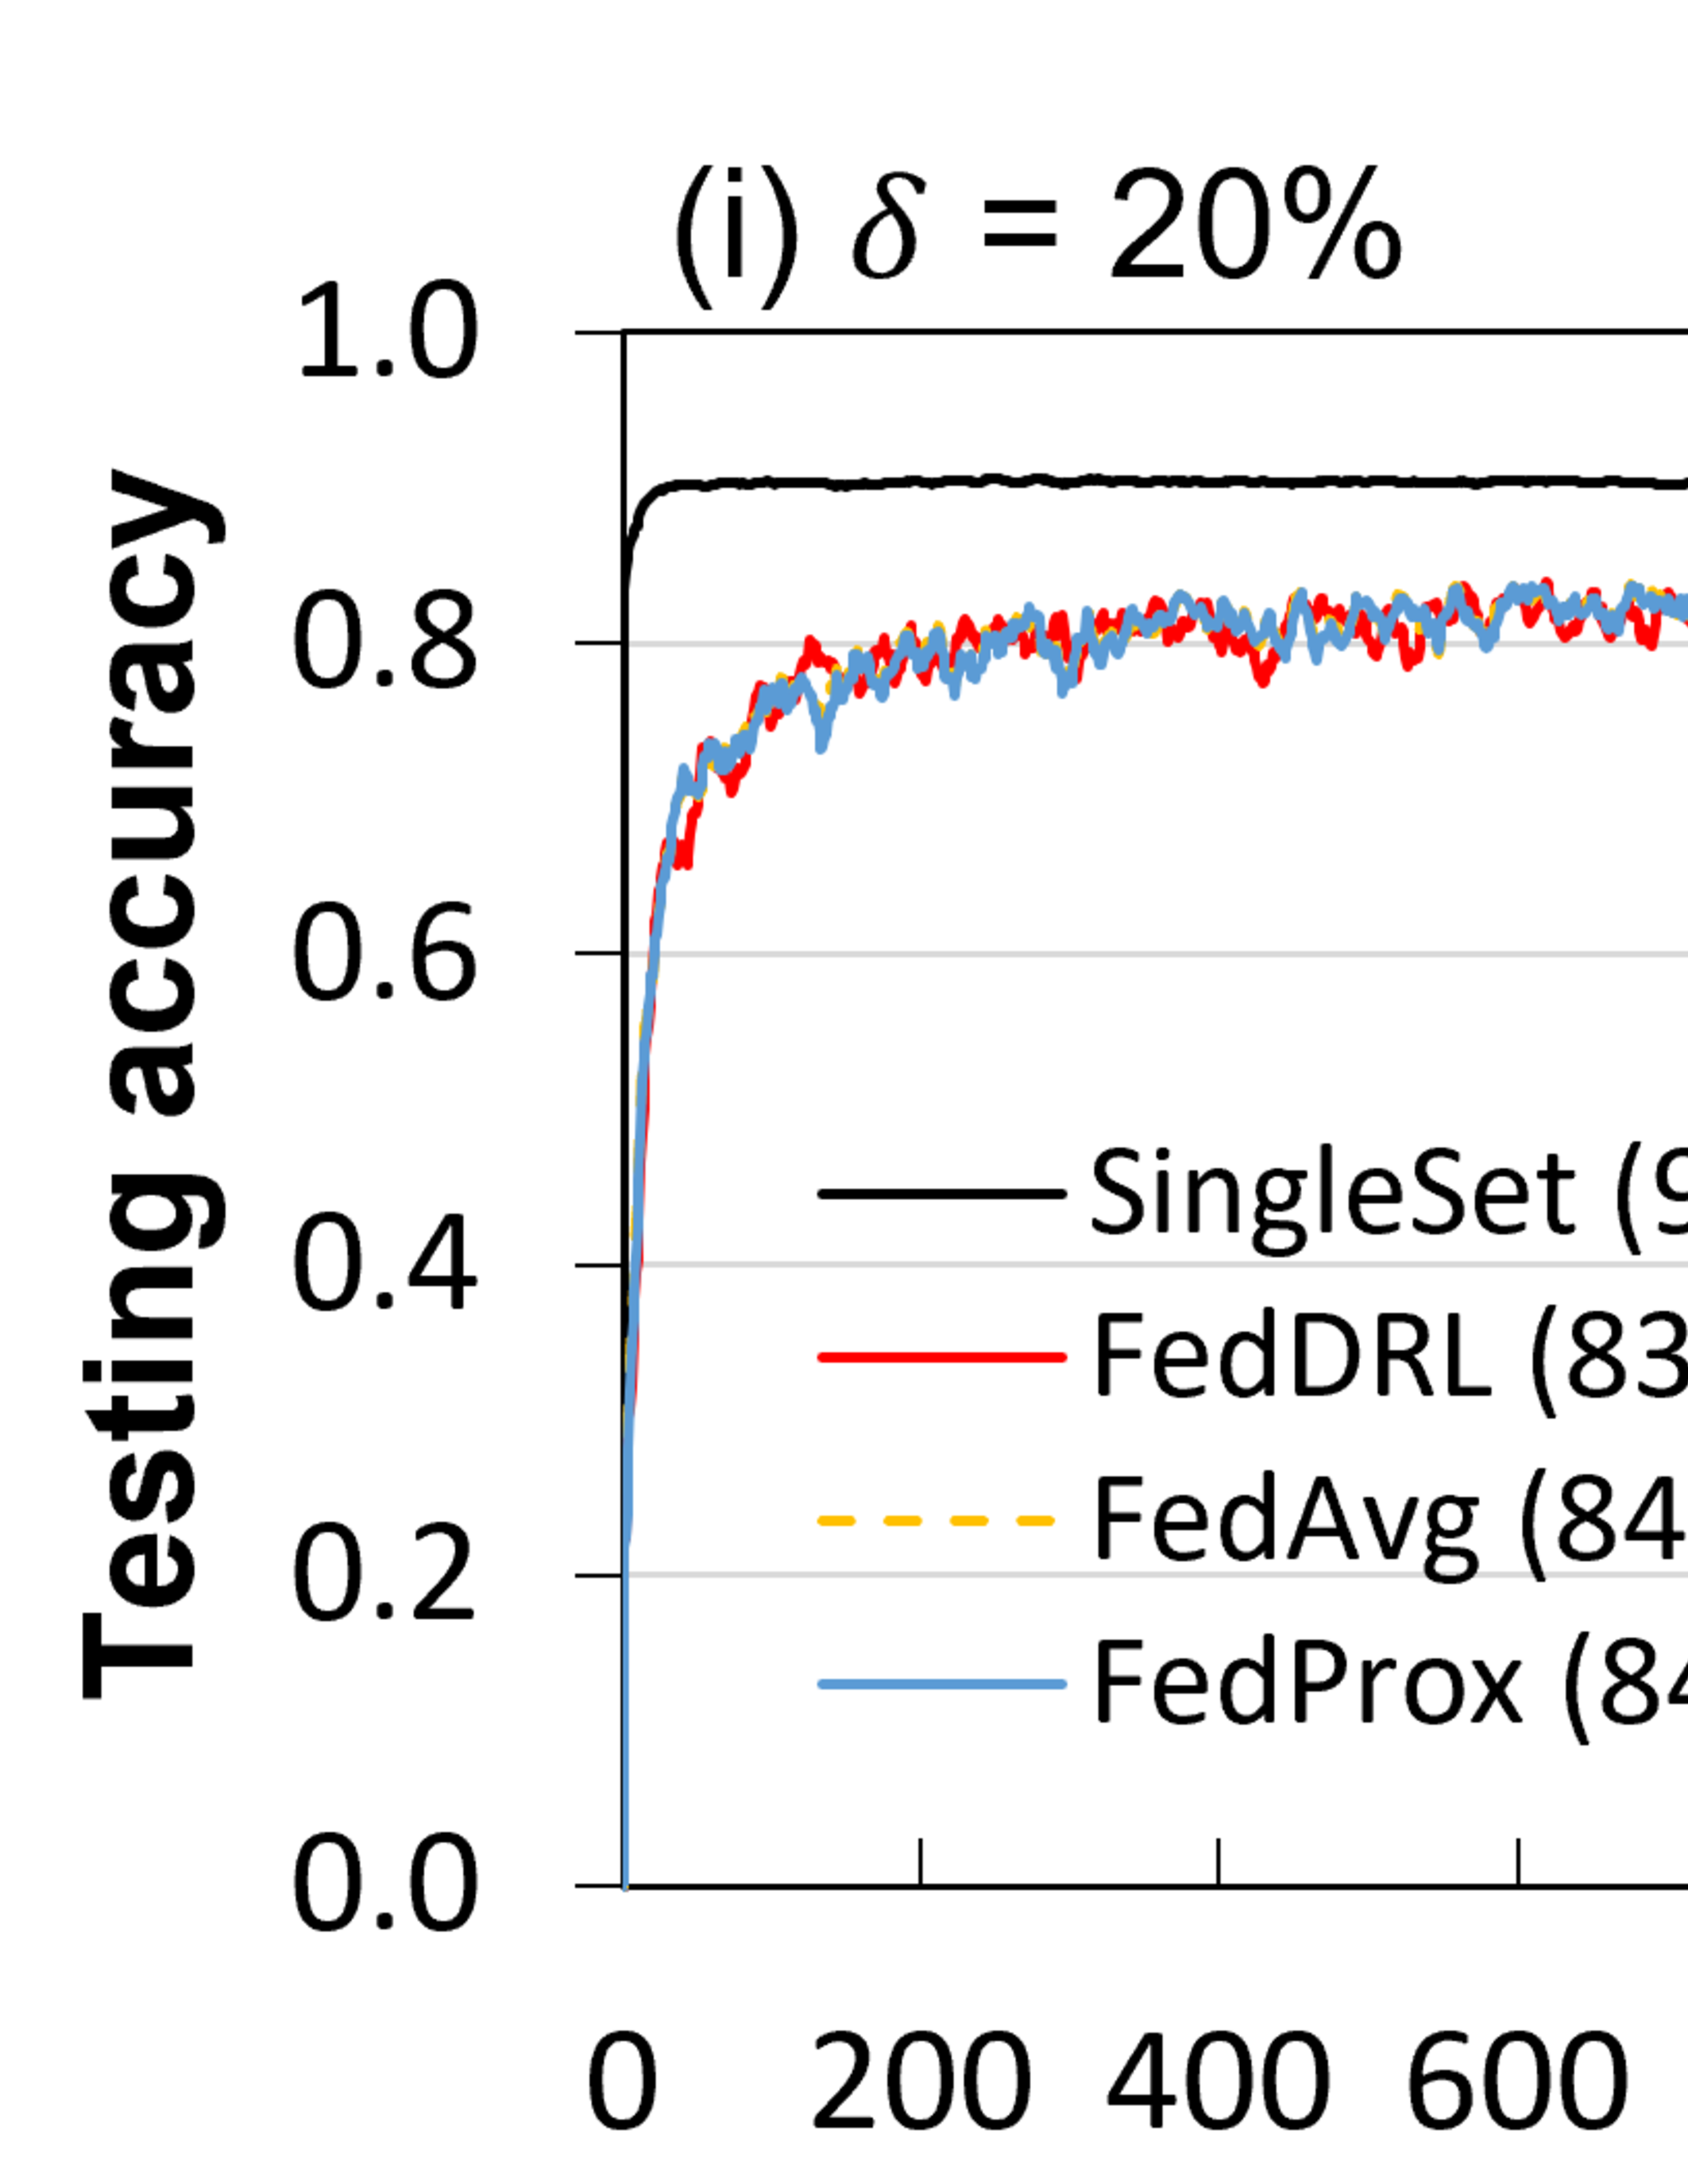}
     }
      \subfigure[Fashion-MNIST, Cluster-NE partitioning, 100 clients.]{
        \label{fig:fmnist_level100_q}
        \includegraphics[width=1\linewidth]{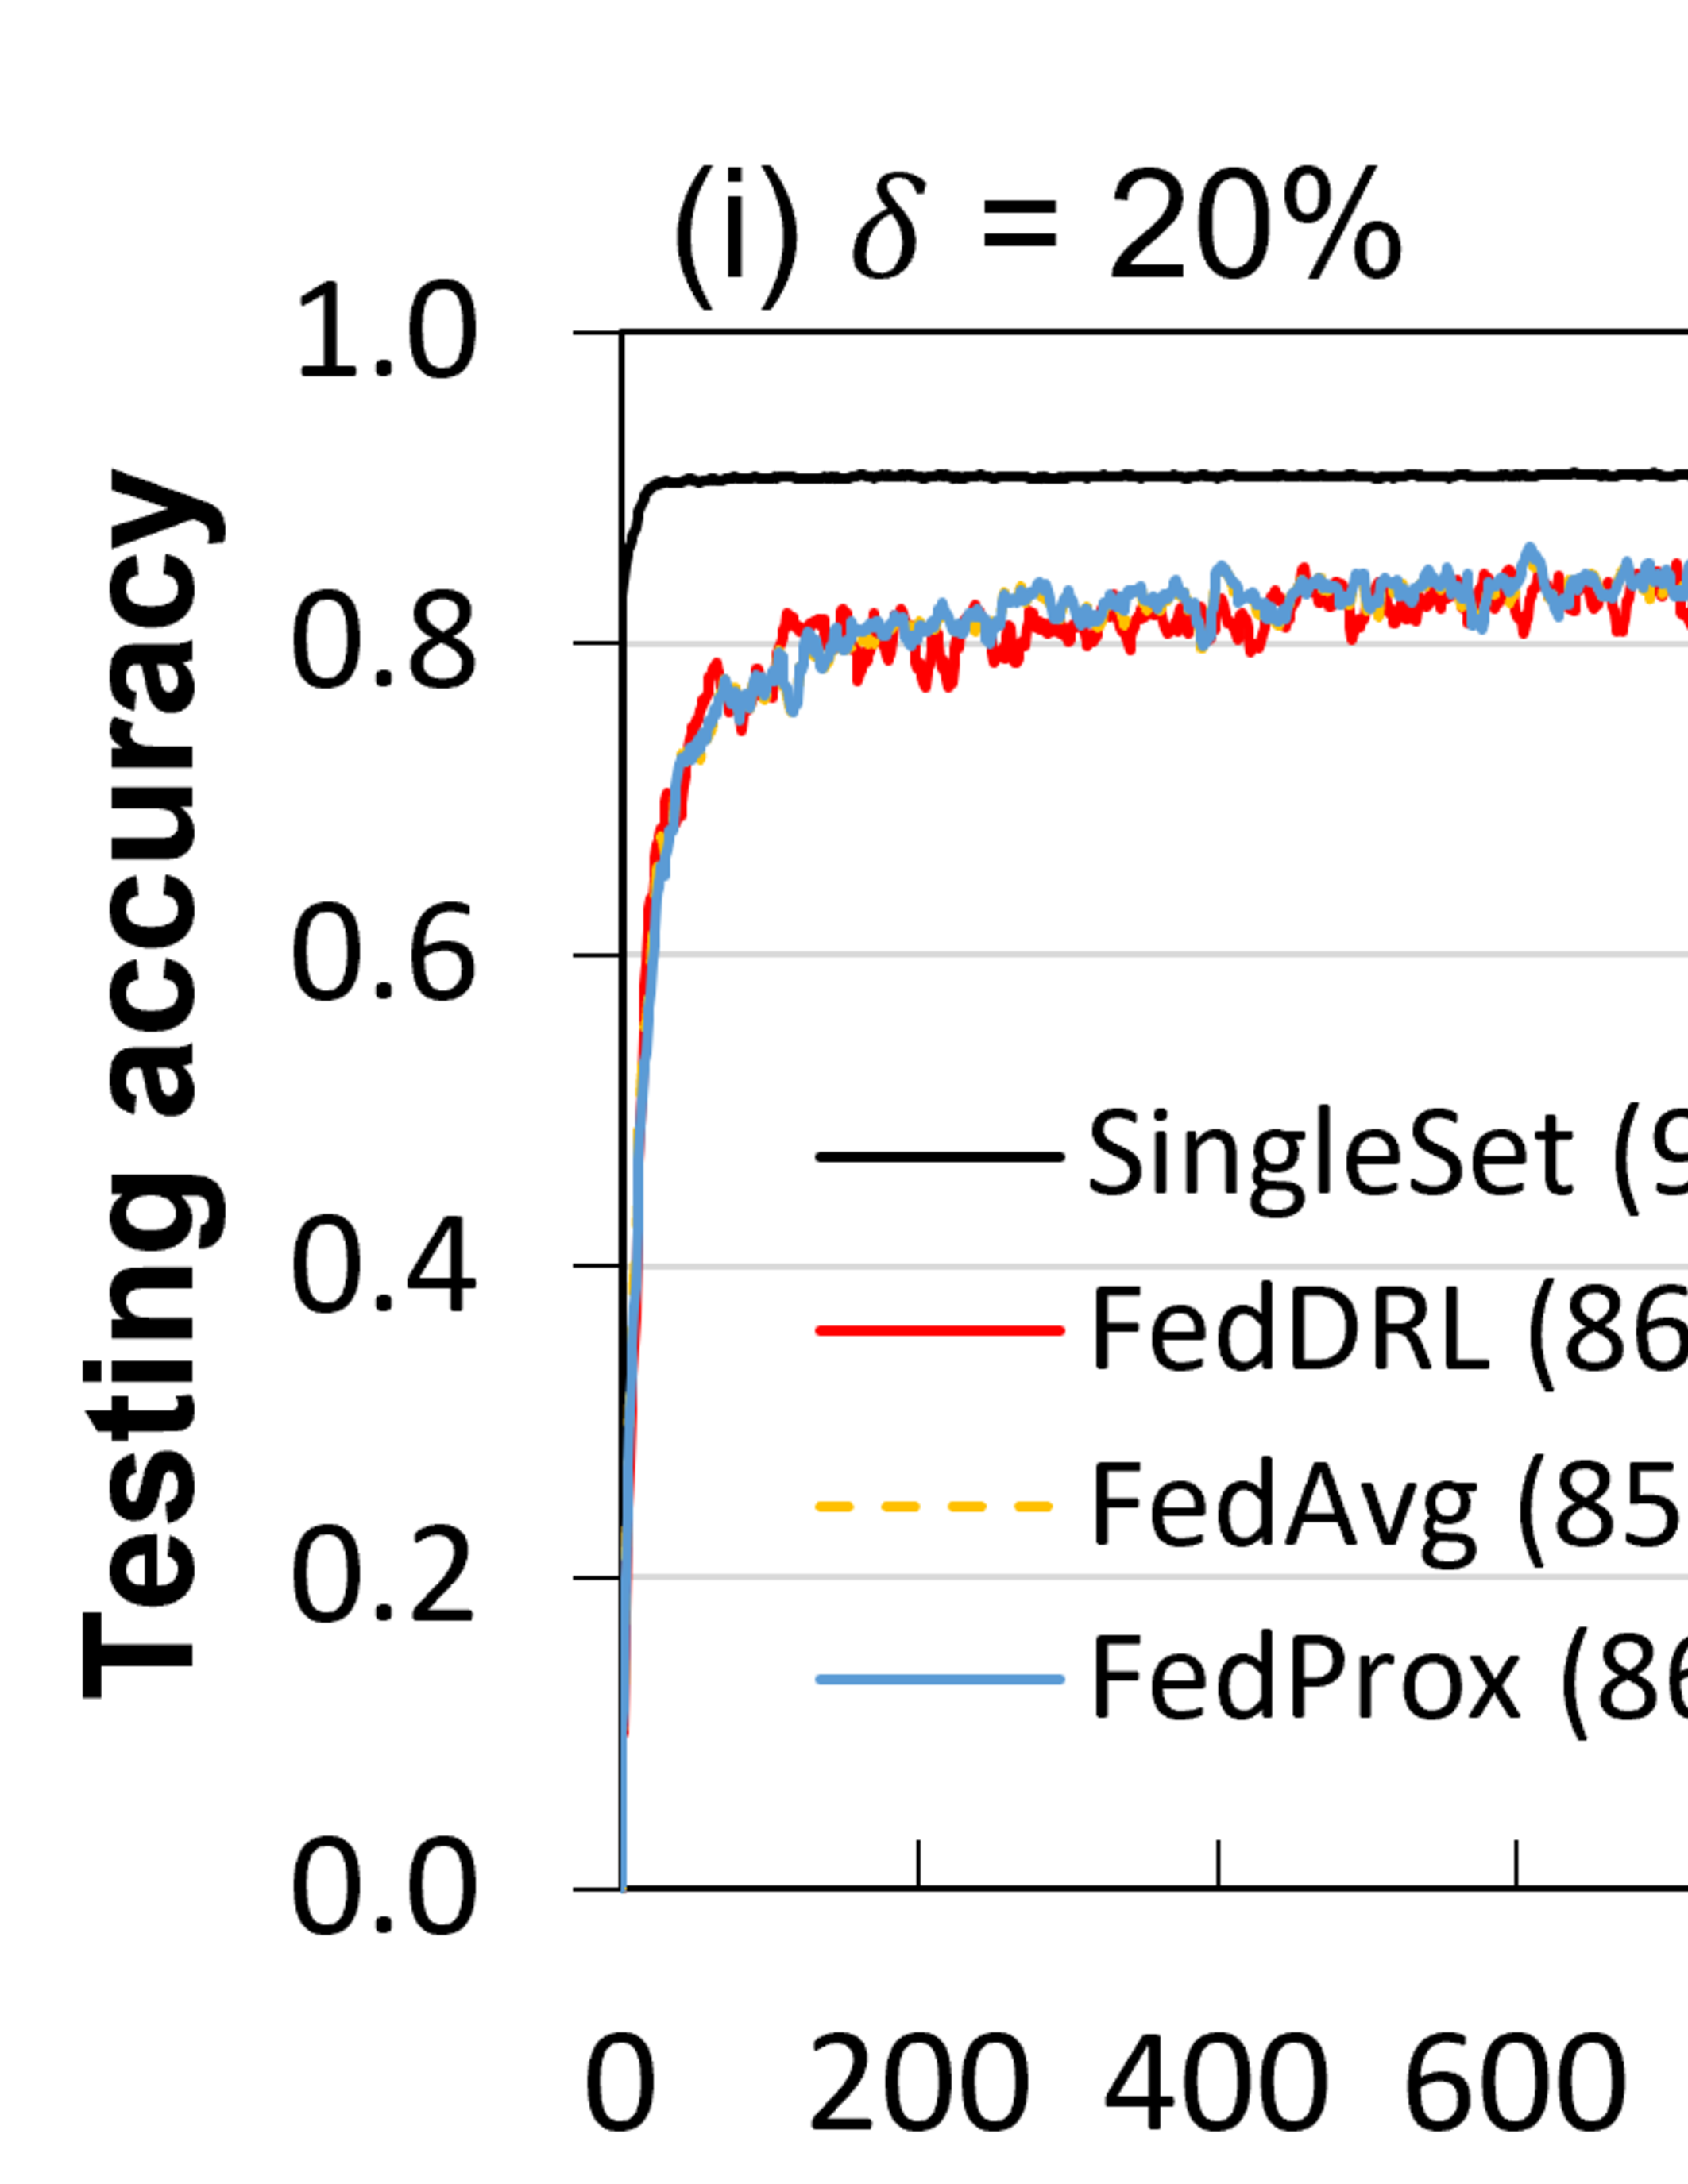}
     }
     \caption{Testing accuracy \textit{vs.} the non-IID level $\delta$ in the case of Fashion-MNIST, 100 clients. The X-axis is communication round. The results are average-smoothed for every $10$ communication round. The values in the legends show the best testing accuracy that each FL methods reach during training.}
     \label{fig:fmnist_level100}
 \end{figure*}

\subsection{Statistic of Partitioned Dataset}
\label{appendix:dataset}

1) Show the table "Statistics of federated datasets
Dataset" ==> For each dataset, each partitioned method, each number of devices, show the total training samples, Mean and STD of samples/devices.
\begin{table}[bt]
	\caption{Statistics of partitioned datasets (01).} 
	\label{table:statistic_dataset_01}
	\centering
	\scriptsize
	\setlength\tabcolsep{3pt} % default value: 6pt
	\resizebox{0.5\textwidth}{!}{%
		\begin{tabular}{lclccccccl}
			\toprule
			\multirow{2}{*}{\textbf{\begin{tabular}[c]{@{}c@{}}Dataset\end{tabular}}} & 
			\multirow{2}{*}{\textbf{\begin{tabular}[c]{@{}c@{}}$\#$clients \end{tabular}}} & 
			\multirow{2}{*}{\textbf{\begin{tabular}[c]{@{}c@{}}Partition \\ Method\end{tabular}}} & 
			\multirow{2}{*}{\textbf{\begin{tabular}[c]{@{}c@{}}$\#$training \\ samples\end{tabular}}} & 
			\multicolumn{2}{c}{\textbf{\begin{tabular}[c]{@{}c@{}}Samples/client\end{tabular}}} &
			\multicolumn{2}{c}{\textbf{\begin{tabular}[c]{@{}c@{}}Classes/client\end{tabular}}}
			\\ \cmidrule(lr){5-6} \cmidrule(lr){7-8}
			& & & & \textbf{mean} & \textbf{std} & \textbf{mean} & \textbf{std} 
			\\ \midrule 
            \multirow{5}{*}{MNIST} & \multirow{5}{*}{10} & Equal & 60000 & 6000 & 0 & 2.7 & 0.48 \\
            & & Non-Equal & 60000 & 6000 & 1414 & 6.4 & 1.43 \\
            & & Pareto & 30858 & 3086 & 3814 & 2 & 0 \\
            & & Clustered-E & 19600 & 1960 & 9 & 2 & 0 \\
            & & Clustered-NE & 24696 & 2470 & 1261 & 2 & 0 \\
            
            \midrule
            \multirow{5}{*}{\begin{tabular}[c]{@{}c@{}}Fashion-\\MNIST\end{tabular}} & \multirow{5}{*}{10} & Equal & 60000 & 6000 & 0 & 1.9 & 0.3  \\
            & & Non-Equal & 60000 & 6000 & 1600 & 4.6 & 1.13 \\
            & & Pareto & 29186 & 2918 & 2517 & 3.3 & 0.78 \\
            & & Clustered-E & 20000 & 2000 & 0 & 2 & 0 \\
            & & Clustered-NE & 19860 & 1986 & 208 & 2 & 0 \\
            
            \midrule
            \multirow{5}{*}{CIFAR-100} & \multirow{5}{*}{10} & Equal & 50000 & 5000 & 0 & 18.9 & 0.7 \\
            & & Non-Equal & 50000 & 5000 & 1047 & 18.7 & 3.57 \\
            & & Pareto & 39550 & 3955 & 3387 & 22.4 & 1.1 \\
            & & Clustered-E & 16000 & 1600 & 0 & 20 & 0 \\
            & & Clustered-NE & 20160 & 2016 & 1029 & 20 & 0 \\
            
            \midrule
            \multirow{5}{*}{MNIST} & \multirow{5}{*}{100} & Equal & 60000 & 600 & 0 & 2 & 0.4 \\
            & & Non-Equal & 60000 & 600 & 147 & 4.71 & 1.25 \\
            & & Pareto & 42876 & 428 & 1081 & 1.91 & 0.8 \\
            & & Clustered-E & 19200 & 192 & 0 & 2 & 0 \\
            & & Clustered-NE & 19050 & 190 & 16 & 2 & 0 \\
            
            \midrule
            \multirow{5}{*}{\begin{tabular}[c]{@{}c@{}}Fashion-\\MNIST\end{tabular}} &  \multirow{5}{*}{100} & Equal & 60000 & 600 & 0 & 1.92 & 0.27 \\
            & & Non-Equal & 60000 & 600 & 151 & 4.62 & 1.06 \\
            & & Pareto & 32444 & 324 & 910 & 1.92 & 0.27 \\
            & & Clustered-E & 20000 & 200 & 0 & 2 & 0 \\
            & & Clustered-NE & 19772 & 197 & 21 & 2 & 0 \\
            
            \midrule
            \multirow{5}{*}{CIFAR-100} &\multirow{5}{*}{100} & Equal & 50000 & 500 & 0 & 3.94 & 0.24 \\
            & & Non-Equal & 50000 & 500 & 179 & 3.94 & 1.40 \\
            & & Pareto & 13910 & 139 & 301 & 4.94 & 0.23 \\
            & & Clustered-E & 24000 & 240 & 0 & 20 & 0 \\
            & & Clustered-NE & 23320 & 233 & 26 & 20 & 0 \\
            
			\bottomrule
		\end{tabular}
	}
	%\vspace{-0.3cm}
\end{table}
\begin{table}[bt]
	\caption{Statistics of partitioned datasets (02).} 
	\label{table:statistic_dataset_02}
	\centering
	\scriptsize
	\setlength\tabcolsep{3pt} % default value: 6pt
	\resizebox{0.5\textwidth}{!}{%
		\begin{tabular}{lclccccccl}
			\toprule
			\multirow{2}{*}{\textbf{\begin{tabular}[c]{@{}c@{}}Dataset\end{tabular}}} & 
			\multirow{2}{*}{\textbf{\begin{tabular}[c]{@{}c@{}}$\#$clients \end{tabular}}} & 
			\multirow{2}{*}{\textbf{\begin{tabular}[c]{@{}c@{}}Partition \\ Method\end{tabular}}} & 
			\multirow{2}{*}{\textbf{\begin{tabular}[c]{@{}c@{}}$\#$training \\ samples\end{tabular}}} & 
			\multicolumn{2}{c}{\textbf{\begin{tabular}[c]{@{}c@{}}Samples/client\end{tabular}}} &
			\multicolumn{2}{c}{\textbf{\begin{tabular}[c]{@{}c@{}}Classes/client\end{tabular}}}
			\\ \cmidrule(lr){5-6} \cmidrule(lr){7-8}
			& & & & \textbf{mean} & \textbf{std} & \textbf{mean} & \textbf{std} 
			\\ \midrule 
            \multirow{5}{*}{MNIST} & \multirow{5}{*}{10} & Equal & 60000 & 6000 & 0 & 2.8 & 0.74 \\
            & & Non-Equal & 60000 & 6000 & 938 & 0.3 & 0.78 \\
            & & Pareto & 25378 & 2537 & 3286 & 2 & 0 \\
            & & Clustered-E & 19600 & 1960 & 0 & 2 & 0 \\
            & & Clustered-NE & 27440 & 2744 & 1590 & 2 & 0 \\
            
            \midrule
            \multirow{5}{*}{\begin{tabular}[c]{@{}c@{}}Fashion-\\MNIST\end{tabular}} & \multirow{5}{*}{10} & Equal & 60000 & 6000 & 0 & 1.7 & 0.45  \\
            & & Non-Equal & 60000 & 6000 & 979 & 4.1 & 0.7 \\
            & & Pareto & 11898 & 1189 & 1742 & 2 & 0 \\
            & & Clustered-E & 20000 & 2000 & 0 & 2 & 0 \\
            & & Clustered-NE & 19682 & 1968 & 153 & 2 & 0 \\
            
            \midrule
            \multirow{5}{*}{CIFAR-100} & \multirow{5}{*}{10} & Equal & 50000 & 5000 & 0 & 19 & 0.44 \\
            & & Non-Equal & 50000 & 5000 & 552 & 18.8 & 2.31 \\
            & & Pareto & 43550 & 4355 & 3904 & 22.8 & 1.07 \\
            & & Clustered-E & 16000 & 1600 & 0 & 20 & 0 \\
            & & Clustered-NE & 20160 & 2016 & 1029 & 20 & 0 \\

            \midrule
            \multirow{5}{*}{CIFAR-100} &\multirow{5}{*}{100} & Equal & 50000 & 500 & 0 & 4.9 & 0.3 \\
            & & Non-Equal & 50000 & 500 & 174 & 3.96 & 1.36 \\
            & & Pareto & 10135 & 101 & 242 & 4.87 & 0.33 \\
            & & Clustered-E & 16000& 160 & 0 & 20 & 0 \\
            & & Clustered-NE & 15920 & 159 & 51 & 20 & 0 \\
            
			\bottomrule
		\end{tabular}
	}
	%\vspace{-0.3cm}
\end{table}
\begin{table}[bt]
	\caption{Statistics of partitioned datasets (03).} 
	\label{table:statistic_dataset_03}
	\centering
	\scriptsize
	\setlength\tabcolsep{3pt} % default value: 6pt
	\resizebox{0.5\textwidth}{!}{%
		\begin{tabular}{lclccccccl}
			\toprule
			\multirow{2}{*}{\textbf{\begin{tabular}[c]{@{}c@{}}Dataset\end{tabular}}} & 
			\multirow{2}{*}{\textbf{\begin{tabular}[c]{@{}c@{}}$\#$clients \end{tabular}}} & 
			\multirow{2}{*}{\textbf{\begin{tabular}[c]{@{}c@{}}Partition \\ Method\end{tabular}}} & 
			\multirow{2}{*}{\textbf{\begin{tabular}[c]{@{}c@{}}$\#$training \\ samples\end{tabular}}} & 
			\multicolumn{2}{c}{\textbf{\begin{tabular}[c]{@{}c@{}}Samples/client\end{tabular}}} &
			\multicolumn{2}{c}{\textbf{\begin{tabular}[c]{@{}c@{}}Classes/client\end{tabular}}}
			\\ \cmidrule(lr){5-6} \cmidrule(lr){7-8}
			& & & & \textbf{mean} & \textbf{std} & \textbf{mean} & \textbf{std} 
			\\ \midrule 
            \multirow{5}{*}{MNIST} & \multirow{5}{*}{10} & Equal & 60000 & 6000 & 0 & 2.7 & 0.64 \\
            & & Non-Equal & 60000 & 6000 & 938 & 7.1 & 0.94 \\
            & & Pareto & 22470 & 2247 & 20254 & 2 & 0 \\
            & & Clustered-E & 19600 & 1960 & 0 & 2 & 0 \\
            & & Clustered-NE & 27440 & 2744 & 1589 & 2 & 0 \\
            
            \midrule
            \multirow{5}{*}{\begin{tabular}[c]{@{}c@{}}Fashion-\\MNIST\end{tabular}} & \multirow{5}{*}{10} & Equal & 60000 & 6000 & 0 & 2 & 0 \\
            & & Non-Equal & 60000 & 6000 & 1131 & 4.2 & 0.97 \\
            & & Pareto & 16718 & 1671 & 2080 & 1.9 & 0.3 \\
            & & Clustered-E & 20000 & 2000 & 0 & 2 & 0 \\
            & & Clustered-NE & 21438 & 2143 & 287 & 2 & 0 \\
            
            \midrule
            \multirow{5}{*}{CIFAR-100} & \multirow{5}{*}{10} & Equal & 50000 & 5000 & 0 & 19.2 & 0.74 \\
            & & Non-Equal & 50000 & 5000 & 645 & 18.6 & 2.37 \\
            & & Pareto & 39775 & 3977 & 3160 & 23.1 & 1.44 \\
            & & Clustered-E & 16000 & 1600 & 0 & 20 & 0 \\
            & & Clustered-NE & 20160 & 2016 & 1029 & 20 & 0 \\

            \midrule
            \multirow{5}{*}{CIFAR-100} &\multirow{5}{*}{100} & Equal & 50000 & 500 & 0 & 4.89 & 0.31 \\
            & & Non-Equal & 50000 & 500 & 146 & 38.9 & 9.35 \\
            & & Pareto & 14270 & 142 & 289 & 4.97 & 0.17 \\
            & & Clustered-E & 16000 & 160 & 0 & 20 & 0 \\
            & & Clustered-NE & 16060 & 160 & 56 & 20 & 0 \\
            
			\bottomrule
		\end{tabular}
	}
	%\vspace{-0.3cm}
\end{table}
